# Supplementary material for: Is an Object-Centric Video Representation Beneficial for Transfer?
Source: arXiv:2207.10075 source file (2022-10-08)
Supplement: Supplementary file 1 [file aux.tex]

\section{Other auxiliary losses}
We have tried applying some other types of auxiliary losses on the object summary output from our Object Learner. 
Results (\Cref{tab:auxloss}) show that they do not help achieve a better performance on downstream tasks, hence are not included in the main paper. 
We list them below as supplementary materials.
% Here we listed different types of losses we have explored and their performance on action recognition and hand contact state detection.
% According to our experiment results, they do not help achieve better results on downstream tasks than having single instance-level contrastive loss on object trajectories.
\subsection{Instance-level contrastive loss on visual affinity vectors}
Given the visual feature maps of a clip and the bounding boxes of an object in it, 
we ROI-Pool the object features $w_j$ from each frame, where j is the index of object. Using these per-frame object features, we compute the transformation vectors between frames:

\begin{equation}
    \mathbf{\tilde{aff}}^i_j =
    \mathbf{w}^i_j \cdot \mathbf{\transpose{w}}^{i+1}_j ,
\end{equation}
We embed the transformation vectors of an object along the temporal dimension into one feature vector $z_j$ and its shuffled version $z^{shuffle}_j$. The encoding is done by using a small Transformer $g(.)$ with 2 layers and 4 heads.
\begin{equation}
    \mathbf{z_j} = g(\mathbf{\tilde{aff}}_j),
\end{equation}
\begin{equation}
    \mathbf{z}^{shuffle}_j = g(\mathbf{\tilde{aff}}^{shuffle}_j),
\end{equation}
\begin{equation}
\mathbf{\tilde{aff}}_j= (\mathbf{\tilde{aff}}^1_j, \mathbf{\tilde{aff}}^2_j, \hdots,\mathbf{\tilde{aff}}^{T'-1}_{j})
\end{equation}
\begin{equation}
    \mathbf{\tilde{aff}}^{shuffle}_j= Shuffle(\mathbf{\tilde{aff}}^1_j, \mathbf{\tilde{aff}}^2_j, \hdots,\mathbf{\tilde{aff}}^{T'-1}_{j})
\end{equation}
$z_j$ and $z^{shuffle}_j$ are used in the contrastive loss against object summary vectors $s_j$ as in:
\begin{equation}
    \mathcal{L}_{aff}=-\sum_{j}\Bigg[\log{\frac{ \exp(\transpose{s}_{j} \cdot {z}_{j} ) }
        {\sum_{k}{\exp(\transpose{s}_{j} \cdot {z}_{k})}+ \sum_{k}{\exp(\transpose{s}_{j} \cdot {z}^{shuffle}_{k})} } }\Bigg] 
    \label{eq:aux-aff}
\end{equation}
    


\subsection{Class-level contrastive loss on ROI-Pooled object vectors}
For each object $j$, we know the action class label $l$ it is associated with. 
We apply a supervised contrastive loss on each object summary vector $s_j$,
where other vectors with the same class label $l$ are treated as its positive samples, with different class labels are treated as negative samples.

\begin{equation}
    \mathcal{L}_{obj}=-\sum_{j}\Bigg[\log{\frac{\sum_{k}\exp(\transpose{s}_{j,l} \cdot {s}_{k,l} ) }
        {\sum_{k}\exp(\transpose{s}_{j,l} \cdot {s}_{k,l}) + \sum_{m,l'\neq l}{\exp(\transpose{s}_{j,l} \cdot {s}_{m,l'})} } }\Bigg] 
    \label{eq:aux-obj}
\end{equation}

\begin{table}[]
    \centering
    \resizebox{0.6\textwidth}{!}{%
    \begin{tabular}{c|c|c|l}
    \textbf{Loss}                   & \textbf{OL only} & \textbf{Backbone only} & \textbf{Final} \\ \hline
    $L_{traj}$                     &   71.0      &    72.0           &   73.6    \\
    $L_{traj} + L_{aff}$           &  71.0       &   72.1            &    73.5   \\
    $L_{traj} + L_{aff} + L_{obj}$ &  70.0       &    72.2           &    73.2   \\ \hline
    \end{tabular}%
    }
    \vspace{2mm}
    \caption{\textbf{Ablation on different types of auxiliary losses on SomethingElse.} Adding other auxiliary losses do not improve the action classification results. We choose to use a single contrastive loss on trajectories (Eq.1 in main paper) for simplicity.}
    \label{tab:auxloss}
    \end{table}
